# Supplementary material for: Novel circuit design for high-impedance and non-local electrical measurements of two-dimensional materials
Source: arXiv:1801.10135 ancillary file (2018-01-30)
Supplement: Supplementary file 1 [file SUPPLEMENTARY_paper_Optocouplers_AdeS.pdf]

## SUPPLEMENTARY INFORMATION

### Novel circuit design for high-impedance and non-local electrical measurements of two-dimensional materials

Adolfo De Sanctis,<sup>1</sup> Jake D. Mehew,<sup>1</sup> Saad Fadhil Ramadhan,<sup>1,2</sup> Callum P. Tate,<sup>1</sup> Ashley White,<sup>1</sup> Adam R. Woodgate,<sup>1</sup> Monica F. Craciun,<sup>1</sup> and Saverio Russo<sup>1, a)</sup>

<sup>1)</sup>*Centre for Graphene Science, College of Engineering,  
Mathematics and Physical Sciences, University of Exeter, Exeter EX4 4QF,  
United Kingdom*

<sup>2)</sup>*Department of Physics, College of Science, University of Duhok, Duhok,  
Kurdistan Region, Iraq*

---

<sup>a)</sup>Correspondence should be addressed to: S.Russo@exeter.ac.uk

TABLE S1. Components list.

|                | V1             |                                      | V2             |                                            |
|----------------|----------------|--------------------------------------|----------------|--------------------------------------------|
| NAME           | VALUE          | TYPE                                 | VALUE          | TYPE                                       |
| R1, R2, R5     | 180 k $\Omega$ | 1% Carbon                            | 180 k $\Omega$ | 0.1% Metal film                            |
| R3, R4         | 680 $\Omega$   | 1% Carbon                            | 680 $\Omega$   | 0.1% Metal film                            |
| VR1, VR2       | 50 k $\Omega$  | 1% Trimmer                           | 50 k $\Omega$  | 1% Trimmer                                 |
| C1, C2, C3     | 10 pF          | Ceramic                              | 10 pF          | $\pm 0.5$ pF Mica                          |
| C4, C5, C7, C8 | 10 $\mu$ F     | Electrolytic                         | 10 $\mu$ F     | Hi-grade Electrolytic                      |
| C6, C9         | 1 $\mu$ F      | Electrolytic                         | 1 $\mu$ F      | Hi-grade Electrolytic                      |
| D1, D2         | 1N4148         | Small signal silicon diode           | 1N4148         | Small signal silicon diode                 |
| IC1, IC2, IC3  | LT1097         | Low-cost, Low Power Precision Op-Amp | LT1028         | Ultralow Noise High Speed Precision Op-Amp |
| IC4, IC5       | ICL7660A       | CMOS Voltage Converter               | ICL7660A       | CMOS Voltage Converter                     |
| OC1, OC2       | HCNR201        | High-Linearity Analog Optocoupler    | HCNR201        | High-Linearity Analog Optocoupler          |
| BAT1, BAT2     | 12 V           | 4Ah LiPo Battery                     | 12 V           | 4Ah LiPo Battery                           |

## I. COMPONENTS LIST AND PCB PROTOTYPES

In table S1 we report the list of components chosen for the realisation of the circuit shown in figure 1 main text in the two versions.

In figure S2a we show the physical realisation of the optocouplers on printed circuit boards (PCBs) in the two versions (the same PCB is used for both). The circuit is then mounted in an aluminium box and connected to the two batteries as shown in figure S2b. Figure S2c shows the PET vacuum flange (see also figure 2a main text) used to house the SMA connectors from the device under test.

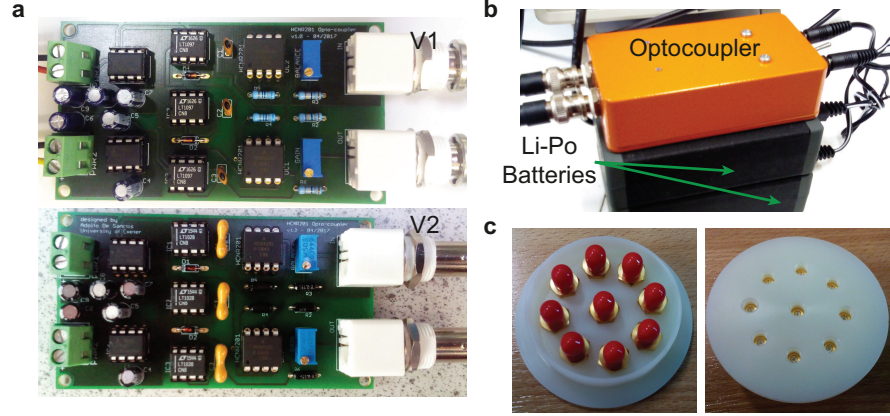

FIG. S2. **PCBs and construction of the optocouplers.** **a**, Assembled PCBs of the V1 (top) and V2 (bottom) optocouplers. **b**, Prototype enclosure and wiring. **c**, Custom-built PET vacuum flange with SMA connectors.
